# Supplementary material for: Meta-RL with Bayesian Linear Task Models
Source: arXiv:2512.20974 source file (2026-11-17)
Supplement: Supplementary file 1 [file appendix.tex]

\newpage
\section{Appendix}
\subsection{Table of Important Notations}
\begin{table}[h]
  \centering
  \label{tab:notation}
  \small
  
  \begin{tabular}{@{}p{0.26\linewidth}p{0.69\linewidth}@{}}
    \toprule
    \textbf{Symbol} & \textbf{Meaning} \\
    \midrule
    \multicolumn{2}{@{}l}{\emph{MDPs and BAMDPs}}\\
    $\mathcal{M}=(S,A,R,T,\gamma)$            & MDP with state space $S$, action space $A$, reward $R$, transition $T$, discount $\gamma$. \\
    $S^{+}=S\times \mathcal{B}_{T}\times \mathcal{B}_{R}$         & BAMDP hyper-state space; $B_{T},B_{R}$ are the belief spaces of $\theta_{T},\theta_{R}$. \\
    $b_{t}=p(\theta_{T},\theta_{R})$          & Belief at time $t$ over task parameters. \\
    $\tau$                                    & Belief-update function, $b_{t+1}=\tau(b_{t},s_{t},a_{t},s_{t+1},r_{t+1})$. \\
    $\pi^{+}_{\psi}(a\mid s,b)$               & BAMDP (BRL) policy parameterised by $\psi$. \\
    $H^{+}$, $\mathcal{J}^{+}(\pi^{+})$                 & BAMDP horizon and expected return. \\
    \midrule
    \multicolumn{2}{@{}l}{\emph{Datasets and dimensions}}\\
    $c_{t}=(s_{t},a_{t},s_{t+1},r_{t+1})$     & Single sample at timestep $t$. \\
    $\mathcal{C}^{\mathcal{M}}=\{c_{t}\}_{t=1}^{N}$     & $N$ samples collected within MDP $\mathcal{M}$. \\
    $\mathcal{C}=\bigcup_{i=1}^{M} \mathcal{C}^{\mathcal{M}_{i}}$ & Joint dataset over a batch of $M$ MDPs. \\
    $\mathcal{C}^{\mathcal{M}_{i}}=(\mathbf{S}_{i},\mathbf{A}_{i},\mathbf{S}'_{i},\mathbf{r}_{i})$ & Samples in compact matrix forms. \\
    $D_{S},\,D_{A}$                           & State and action dimensions. \\
    $D_{T},\,D_{R}$                           & Transition and reward task dimensions. \\
    $D_{P}$                                   & Task-representation dimension. \\
    \midrule
    \multicolumn{2}{@{}l}{\emph{Task parameters}}\\
    $\theta_{T}=(T_{\mu},T_{\sigma})$         & Transition task parameter: mean $T_{\mu}$, noise covariance $T_{\sigma}$. \\
    $\theta_{R}=(R_{\mu},R_{\sigma})$         & Reward task parameter: mean $R_{\mu}$, noise covariance $R_{\sigma}$. \\
    \midrule
    \multicolumn{2}{@{}l}{\emph{Learnable basis functions}}\\
    $\phi_{T},\,\phi_{R}$                     & Neural networks acting as basis functions for transition and reward. \\
    $\mathbf{C}_{T}=\phi_{T}(S_{i},A_{i})$ & Transition features (design matrix). \\
    $\mathbf{C}_{R}=\phi_{R}(S_{i},A_{i},S'_{i})$ & Reward features (design matrix). \\
    $\zeta$                                   & Optional network parameterising the prior $p_{\zeta}(\theta_{T},\theta_{R})$. \\
    \midrule
    \multicolumn{2}{@{}l}{\emph{Distributions}}\\
    $\mathcal{MN}(\mathbf{W}\mid \mathbf{X},\mathbf{Y},\mathbf{Z})$               & Matrix-normal: mean $\mathbf{X}$, row covariance $\mathbf{Y}$, column covariance $\mathbf{Z}$. \\
    $\mathcal{W}(\mathbf{W}\mid \mathbf{X},\nu)$                & Wishart: scale matrix $\mathbf{X}$, degrees of freedom $\nu$. \\
    \midrule
    \multicolumn{2}{@{}l}{\emph{Prior/posterior parameters}}\\
    $\Mt$/$\Mt'$  & Prior/posterior mean of $T_{\mu}$. \\
    $\xit^{-1}$/${\xit'}^{-1}$ & Prior/posterior row covariance of $T_{\mu}$ ($\xit$ is the row precision). \\
    $\omegat$/$\omegat'$, $\nut$/$\nut'$ & Prior/posterior Wishart scale and dof on $T_{\sigma}^{-1}$. \\
            & Parameters for $\theta_{R}$ follow analogously. \\
    \midrule
    \multicolumn{2}{@{}l}{\emph{Kernel-correspondence}}\\
    $k_{TT},\,k_{R},\,k_{TTR}$                & Kernel functions induced by the learnt basis (defined in \Apref{theory}). \\
    $w_{TT},\,w_{R},\,w_{TTR}$                & Associated weighting functions. \\
    $\mathrm{sCMS}^{w}_{k}(\mathcal{C}^{\mathcal{M}_{1}},\mathcal{C}^{\mathcal{M}_{2}})$ & Empirical signed-measure Cosine Mean Similarity. \\
    $\mathrm{sMMD}^{w}_{k}(\mathcal{C}^{\mathcal{M}_{1}},\mathcal{C}^{\mathcal{M}_{2}})$ & Empirical signed-measure Maximum Mean Discrepancy. \\
    \bottomrule
  \end{tabular}
\end{table}
\newpage

\subsection{\nom Algorithm}
\begin{algorithm}[h]
    \caption{\nom \label{glibrlalg}}

    Initialise: policy $\pi^+_{\psi}$, horizon $H$, $\phit, \phir$\;
    \While {Training}{
        Sample $K$ MDPs $\left\{\mathcal{M}_i\right\}_{i=1}^{K}$\;
        Initialise: Joint data $\mathcal{C} = \{\}$\;
        \tcp{collecting samples}
        \For {$i \in \{1, 2, \cdots, K\}$}{
            Initialise: samples in ${\mathcal{M}_i}$,  $\mathcal{C}^{\mathcal{M}_i} = \{\}$, state $s$\; 

            \For{$t < H$} {
                $b \gets p_{\phit, \phir}({\thetat}, {\thetar} | \mathcal{C}^{\mathcal{M}_i})$\;
                $a \sim \pi_{\psi}^{+} (a|s, b)$\;
                Execute $a$ from $s$ in $\mathcal{M}_i$ to get $s', r$\;
                $\mathcal{C}^{\mathcal{M}_i} \gets \mathcal{C}^{\mathcal{M}_i} \cup \{s, a, s', r\}$\;
                $s \gets s'$\;
            }
            $\mathcal{C} =\mathcal{C} \cup \mathcal{C}^{\mathcal{M}_i}$
        }
        \tcp{learning policy, transition and reward models}
        \While{Learning}{
            Sample $\mathcal{D} \subseteq \mathcal{C}$\;
            $\psi \gets \psi - \nabla_{\psi} \mathcal{L}_{\text{policy}}(\mathcal{D})$\;
            $\phit \gets \phit - \nabla_{\phit} \mathcal{L}_{\text{model}}(\mathcal{D})$\;
            $\phir \gets \phir - \nabla_{\phir} \mathcal{L}_{\text{model}}(\mathcal{D})$\;
        }
    }
\end{algorithm}
\vspace{-1em}

\subsection{GLiBRL-SAC}
\begin{algorithm}[h]
    \caption{GLiBRL with SAC \label{alg:glibrl_sac}}
    \While {Training}{
    \tcp{collecting samples following \Algref{glibrlalg}}
        \While{Learning}{
            Sample $\mathcal{D} \subseteq \mathcal{C}$ of \textbf{variable-length} $N \in [1, \mathrm{Horizon}]$ \;
            $b \gets p_{\phit, \phir}({\thetat}, {\thetar} | \mathcal{D})$\;
            $\psi \gets \psi - \nabla_{\psi} (\mathcal{L}_{\text{actor}}(\mathcal{D}, b) + \mathcal{L}_{\text{critic}}(\mathcal{D}, b) + \mathcal{L}_{\alpha})$\;
            Polyak averaging for target Q-networks within $\psi$\;
            \tcp{Model updates following \Algref{glibrlalg}}
        }
    }
\end{algorithm}
\vspace{-1em}

\subsection{GLiBRL-PPO}
\begin{algorithm}[h]
    \caption{GLiBRL with PPO \label{alg:glibrl_ppo}}
    \While {Training}{
        \tcp{collecting samples following \Algref{glibrlalg}}
        Compute advantages $\hat{A}$ and return targets using $\mathcal{C}$\;
        \While{Learning}{
            Sample $\mathcal{D} \subseteq \mathcal{C}$ of \textbf{fixed length} $N$\;
            $\left\{b_i\right\}_{i=1}^N \gets \left\{p_{\phit, \phir}({\thetat}, {\thetar} | \mathcal{D}[1:i])\right\}_{i=1}^N$\;
            $\psi \gets \psi - \nabla_{\psi} \mathcal{L}_{\text{actor}}\left(\mathcal{D}, \hat{A}, \left\{b_i\right\}_{i=1}^N\right)$\;
            \tcp{Model updates following \Algref{glibrlalg}}
        }
    }
\end{algorithm}
\newpage

\subsection{Evidence Lower Bound}
\label{elboproof}
The evidence lower bound in \Eqref{elbo} is derived as follows
\begin{align*}
    \begin{split}
        \log p_{\phit, \phir}(\mathcal{C}) &= \sum_{i=1}^M\log \iint p(\mathcal{C}^{\mathcal{M}_i}, \thetat, \thetar) \frac{q(\thetat, \thetar|\mathcal{C}^{\mathcal{M}_i})}{q(\thetat, \thetar|\mathcal{C}^{\mathcal{M}_i})} d\thetat d\thetar \\
        &\ge \sum_{i=1}^M \mathbb{E}_{q}\left[\log \frac{p(\thetat, \thetar)}{q(\thetat, \thetar|\mathcal{C}^{\mathcal{M}_i})} + \log p(\mathcal{C}^{\mathcal{M}_i}|\thetat, \thetar)  \right] \\
        &= \sum_{i=1}^M { \mathbb{E}_{q}\left[\log p(\mathcal{C}^{\mathcal{M}_i}|\thetat, \thetar) \right] - D_{KL}\left({q(\thetat, \thetar|\mathcal{C}^{\mathcal{M}_i})} \Vert p(\thetat, \thetar)\right) } 
    \end{split}
\end{align*}

\subsection{Normal-Wishart-Normal Conjugacy}
\label{nwconjugacy}
Given \Eqref{tprior} 
\begin{equation*}
    p(\thetat)  = \mathcal{MN}(\mut|\Mt, \xit^{-1}, \sigmat) \cdot \mathcal{W}(\sigmat^{-1}|\omegat^{-1}, \nut)
\end{equation*}
and \Eqref{tllh}
\begin{align*}
    \recallLabel{tllh}
\end{align*}
We prove \Eqref{tpost} 
\begin{align*}
    \recallLabel{tpost}
\end{align*}
where
\begin{equation*}
    \recallLabel{post}
\end{equation*}
\subsubsection*{Proof:}
The density of the prior distribution $p(\thetat)$ is
\begin{align}
    \begin{split}
        p(\thetat) &=\frac{|\xit|^{D_S/2}}{\sqrt{(2\pi)^{D_TD_S}}|\sigmat|^{D_T/2}} \cdot \exp{\left[ -\frac{1}{2}\Tr\left( \sigmat^{-1} (\mut - \Mt)^\text{T} \xit  (\mut - \Mt) \right) \right]}\\
        & \cdot 
        \sqrt{\frac{|\omegat|^{\nut}}{2^{\nut D_S}}} \frac{|\sigmat|^{(1 + D_S -\nut)/2}}{\Gamma_{D_S}(\nut / 2)} \cdot \exp{\left[ -\frac{1}{2} \Tr{\left( \omegat \sigmat^{-1} \right)}\right]} \label{a210}
    \end{split}\\
    \begin{split}
            &\propto|\sigmat|^{{(1+D_S-\nut - D_T)/2}}  \cdot \exp{\Bigl\{ -\frac{1}{2} \Tr\Bigl[ \sigmat^{-1} \Bigl[(\mut - \Mt)^\text{T} \xit  (\mut - \Mt)  +\omegat \Bigr]\Bigr ] \Bigr\}} \label{a211}
    \end{split}
\end{align}
where from \Eqref{a210} to \Eqref{a211} we treat multiplicative parameters irrelevant to $\thetat$ as constants. The joint density of $p_{\phit}(\thetat, \mathbf{S}_i' | \mathbf{S}_i, \mathbf{A}_i) = p(\thetat) \cdot p_{\phit}(\mathbf{S}_i'|\mathbf{S}_i, \mathbf{A}_i, \thetat)$ is hence
{
\begin{align}
    \begin{split}
           & \frac{|\xit|^{D_S/2}}{\sqrt{(2\pi)^{D_TD_S}}|\sigmat|^{D_T/2}} \cdot \exp{\left[ -\frac{1}{2}\Tr\left( \sigmat^{-1} (\mut - \Mt)^\text{T} \xit  (\mut - \Mt) \right) \right]}\\
            & \cdot 
            \sqrt{\frac{|\omegat|^{\nut}}{2^{\nut D_S}}} \frac{|\sigmat|^{(1 + D_S -\nut)/2}}{\Gamma_{D_S}(\nut / 2)} \cdot \exp{\left[ -\frac{1}{2} \Tr{\left( \omegat \sigmat^{-1} \right)}\right]} \\
            &  \cdot \frac{1}{\sqrt{(2\pi)^{ND_S}}|\sigmat|^{N/2}} \cdot \exp{\left[ -\frac{1}{2} \Tr\left( \sigmat^{-1} (\mathbf{S}_i' - \Ct\mut)^{\text{T}} (\mathbf{S}_i' - \Ct\mut)\right) \right]} \label{a215}
    \end{split} \\[10pt]
    \begin{split}
        &\propto |\sigmat|^{{(1 +D_S-\nut - N - D_T)/2}}  \cdot \exp{\left[ -\frac{1}{2}\Tr\left( \sigmat^{-1} (\mut - \Mt)^\text{T} \xit  (\mut - \Mt) \right) \right]} \\
        & \qquad \qquad \qquad \qquad \cdot\exp{\left[ -\frac{1}{2} \Tr\left( \sigmat^{-1} \left( (\mathbf{S}_i' - \Ct\mut)^{\text{T}} (\mathbf{S}_i' - \Ct\mut) + \omegat\right) \right)  \right]}
        \label{a216}
    \end{split}
\end{align}
}
% \begin{align}
% \propto\; & |\Sigma_t|^{\frac{1-D_S-\nu_t - N - D_T}{2}}
% \exp\!\left\{ -\tfrac{1}{2}\Tr\!\left[
% \Sigma_t^{-1}\Big(
% (\mu_t - M_t)^{\!\top}\,\Xi_t\,(\mu_t - M_t)\right.\right. \nonumber\\
% &\left.\left.\qquad\qquad\qquad
% + (\mathbf{S}_i' - C_t\mu_t)^{\!\top}(\mathbf{S}_i' - C_t\mu_t)
% + \Omega_t
% \Big)\right]\right\}
% \end{align}
Matching the second-order then the first-order term with respect to $\mut$, we can rewrite 
\begin{align}
    \begin{split}
        \text{\ref{a216}} = |\sigmat|^{{(1+D_S-\nut' - D_T)/2}}  \cdot \exp{\Bigl\{ -\frac{1}{2} \Tr\Bigl[ \sigmat^{-1} \Bigl[(\mut - \Mt')^\text{T} \xit'  (\mut - \Mt')  +\omegat' \Bigr]\Bigr ] \Bigr\}} \label{a217}
    \end{split}
\end{align}
We can find \Eqref{a211} and \Eqref{a217} match exactly, indicating the Normal-Wishart-Normal conjugacy. Note, we just use the posterior update of $p(\thetat)$ as an example. The exact same proof applies to the posterior update of $p(\thetar)$ as well. Such conjugacy allows exact posterior update and marginal likelihood, enabling efficient learning.  

\subsection{Marginal Log-likelihood of Normal-Wishart-Normal}
\label{llhproof}
We prove \Eqref{llhour} has the following closed form
\begin{align*}
    \recallLabel{llhour}
\end{align*}

\subsubsection*{Proof:} 

Consider
\begin{equation}
    \begin{split}
        p_{\phit} ( \mathbf{S}_i'|\mathbf{S}_i, \mathbf{A}_i) = \frac{p_{\phit}(\thetat,  \mathbf{S}_i'|\mathbf{S}_i, \mathbf{A}_i)}{p_{\phit}(\thetat|\mathbf{S}_i, \mathbf{A}_i, \mathbf{S}_i')}
    \end{split}
\end{equation}
From \Apref{nwconjugacy}, we know the numerator is

\begin{equation}
    \frac{|\xit|^{D_S/2}  |\omegat|^{\nut/2}} {2^{\nut D_S/2}\cdot(2\pi)^{D_S(D_T+N)/2}\cdot\Gamma_{D_S}(\nut/2)} \cdot \text{\Eqref{a217}}
\end{equation}

The denominator is
\begin{equation}
    \frac{|\xit'|^{D_S/2}  |\omegat'|^{\nut'/2}} {2^{\nut' D_S/2}\cdot(2\pi)^{D_SD_T/2}\cdot\Gamma_{D_S}(\nut'/2)} \cdot \text{\Eqref{a217}}
\end{equation}

Hence,
\begin{equation}
    \begin{split}
        p_{\phit} (\mathbf{S}_i'|\mathbf{S}_i, \mathbf{A}_i) = \frac{1}{(2\pi)^{D_SN/2}} \cdot \frac{|\xit|^{D_S/2}  |\frac{1}{2}\omegat|^{\nut/2} \cdot\Gamma_{D_S}(\nut'/2)}{|\xit'|^{D_S/2}  |\frac{1}{2}\omegat'|^{\nut'/2} \cdot\Gamma_{D_S}(\nut/2)} 
    \end{split}
\end{equation}

Similarly,
\begin{equation}
    \begin{split}
        p_{\phir} (\mathbf{r}_i | \mathbf{S}_i, \mathbf{A}_i, \mathbf{S}_i') = \frac{1}{(2\pi)^{N/2}} \cdot \frac{|\xir|^{1/2}  |\frac{1}{2}\omegar|^{\nur/2} \cdot\Gamma(\nur'/2)}{|\xir'|^{1/2}  |\frac{1}{2}\omegar'|^{\nur'/2} \cdot\Gamma(\nur/2)} 
    \end{split}
\end{equation}

Note that
\begin{equation}
    p_{\phit, \phir}(\mathcal{C}^{\mathcal{M}_i}) = p_{\phit} (\mathbf{S}_i'|\mathbf{S}_i, \mathbf{A}_i) p_{\phir} (\mathbf{r}_i | \mathbf{S}_i, \mathbf{A}_i, \mathbf{S}_i') p(\mathbf{S}_i, \mathbf{A}_i)
\end{equation}

By taking the logarithm, and note the independence of $p(\mathbf{S}_i, \mathbf{A}_i)$ with respect to $\phit, \phir$,
\begin{equation}
    \log p_{\phit, \phir}(\mathcal{C}^{\mathcal{M}_i}) = \log p_{\phit} (\mathbf{S}_i'|\mathbf{S}_i, \mathbf{A}_i) + \log p_{\phir} (\mathbf{r}_i | \mathbf{S}_i, \mathbf{A}_i, \mathbf{S}_i') + \text{const.}
\end{equation}

Sum the above equation on both sides with respect to $i$, then we have \Eqref{llhour}.
% \begin{equation}
%     \begin{split}
%         p_{\phit} (\mathbf{S}_i, \mathbf{A}_i, \mathbf{S}_i') = \int_{\thetat} p(\thetat) p_{\phit}(\mathbf{S}_i'|\mathbf{S}_i, \mathbf{A}_i, \thetat) d\thetat
%     \end{split}
% \end{equation}

\subsection{Choices of Belief Representations}
\label{beliefrep}
We list several candidate $f$s:
{\small
\begin{align*}
    f_1\left(\Mt, \Mr\right) &= \left[\mathrm{vec}\left(\Mt\right)^{\text{T}} \;  \Mr^{\text{T}}\right]^{\text{T}} \qquad\qquad \qquad f_2\left(\Mt, \Mr\right) = \left[\mathrm{tril}\left(\Mt\Mt^{\text{T}}\right)^{\text{T}} \;  \Mr^{\text{T}}\right]^{\text{T}} \\
    f_3\left(\Mt, \Mr\right) &= \left[\mathrm{tril}\left(\Mt^{\text{T}}\Mt\right)^{\text{T}} \;  \Mr^{\text{T}}\right]^{\text{T}}  \quad f_4\left(\Mt, \Mr\right) = \left[\frac{\mathrm{tril}\left(\Mt\Mt^{\text{T}}\right)}{\left\Vert\mathrm{tril}\left(\Mt\Mt^{\text{T}}\right)\right\Vert_2}^{\text{T}} \;  \frac{\Mr^{\text{T}}}{\left\Vert\Mr\right\Vert_2}\right]^{\text{T}} \\
    f_5\left(\Mt, \Mr\right) &= \left[\frac{\mathrm{tril}\left(\Mt^{\text{T}}\Mt\right)}{\left\Vert\mathrm{tril}\left(\Mt^{\text{T}}\Mt\right)\right\Vert_2}^{\text{T}} \;   \frac{\Mr^{\text{T}}}{\left\Vert\Mr\right\Vert_2}\right]^{\text{T}} \qquad f_6\left(\Mt, \Mr\right) = \left[g_T(\Mt)^{\text{T}} \; g_R(\Mr)^{\text{}}\right]^{\text{T}}
\end{align*}}
\noindent \noindent where $\mathrm{tril}(\cdot)$ retrieves the flattened lower triangle of matrices and $g_T(\cdot), g_R(\cdot)$ are neural networks. $f_1$ directly flattens and concatenates the task means, resulting in $D_T \times D_S + D_R$ dimensional representations. $f_2$ and $f_3$ are used for scenarios with large $D_S$ and $D_T$, giving $D_T(D_T+1)/2 + D_R$ and $D_S(D_S+1)/2 + D_R$ dimensional representations respectively. $f_4$ and $f_5$ normalise the representations. $f_6$ suggests learnable belief representations.

$f_1$ to $f_5$ can all be shown to be equivalent to the kernalised empirical correspondence of task samples from proofs in \Apref{theory}. Because of the use of neural networks in $f_6$, it is difficult to show similar correspondence in general. Neural networks in $f_6$ are trained by backprogating the Reinforcement Learning loss. Empirically, we have observed it performing worse than $f_4$, or $f_{T, R}$ defined in \Secref{plearning}.

\subsection{Equivalence of Bayesian Parameter Shift, sMMD and sCMS}
\label{theory}
Consider two arbitrary sets of samples, which come from two tasks $\mathcal{M}_1$ and $\mathcal{M}_2$: 
\begin{align*}
    \mathcal{C}^{\mathcal{M}_1} = \{s_{1i}, a_{1i}, s_{1i+1}, r_{1i+1}\}_{i=1}^M&=\left(\mathbf{S}_1, \mathbf{A}_1, \mathbf{S}'_1, \mathbf{r}_1\right) \\
    \mathcal{C}^{\mathcal{M}_2} = \{s_{2i}, a_{2i}, s_{2i+1}, r_{2i+1}\}_{i=1}^N&=\left(\mathbf{S}_2, \mathbf{A}_2, \mathbf{S}'_2, \mathbf{r}_2\right)
\end{align*}
and corresponding features 
\begin{align*}
    \Ct^1 = \phit(\mathbf{S}_1, \mathbf{A}_1) \qquad \Cr^1 = \phir(\mathbf{S}_1, \mathbf{A}_1, \mathbf{S}'_1) \qquad
    \Ct^2 = \phit(\mathbf{S}_2, \mathbf{A}_2) \qquad \Cr^2 = \phir(\mathbf{S}_2, \mathbf{A}_2, \mathbf{S}'_2)
\end{align*}
Define the \nom task posterior means ${\Mt^1}'$, ${\Mr^1}'$, ${\Mt^2}'$, ${\Mr^2}'$, assuming shared prior means $\Mt = \mathbf{0}$, $\Mr = \mathbf{0}$ and covariances $\xit$, $\xir$, where the posterior update follows \Eqref{post}. Note that the zero prior mean is only assumed for notational conciseness but not necessary. For example, let $\Ct^{\text{T}}\mathbf{S'} + \xit\Mt = \begin{bmatrix}
    \Ct^{\text{T}} & \mathbf{I}
\end{bmatrix} \begin{bmatrix}
    {\mathbf{S}'}^{\text{T}} & {\Mt^{\text{T}}\xit}
\end{bmatrix}^\text{T} = \widehat{\mathbf{C}_T}^{\text{T}} \widehat{\mathbf{S}'}$. One can proceed with $\widehat{\mathbf{C}_T}$ and $\widehat{\mathbf{S}'}$ following similar proofs to be introduced shortly.

Define functions $w(\cdot)$ mapping from $\mathcal{C}^{\mathcal{M}_1}$ and $\mathcal{C}^{\mathcal{M}_2}$ to vectors. We define the empirical signed-measure Maximum-Mean Discrepancy ($\mathrm{sMMD}$) between $\mathcal{C}^{\mathcal{M}_1}$ and $\mathcal{C}^{\mathcal{M}_2}$ under kernel function $k(\cdot,\cdot)$ and signed weighting function $w(\cdot)$ as
\begin{multline}
    \mathrm{sMMD}_{k}^w\left(\mathcal{C}^{\mathcal{M}_1}, \mathcal{C}^{\mathcal{M}_2}\right) = w\left(\mathcal{C}^{\mathcal{M}_1}\right)^{\text{T}}\mathbf{K}_{11}w\left(\mathcal{C}^{\mathcal{M}_1}\right) + w\left(\mathcal{C}^{\mathcal{M}_2}\right)^{\text{T}}\mathbf{K}_{22}w\left(\mathcal{C}^{\mathcal{M}_2}\right) \\ - 2w\left(\mathcal{C}^{\mathcal{M}_1}\right)^{\text{T}}\mathbf{K}_{12}w\left(\mathcal{C}^{\mathcal{M}_2}\right)
\end{multline}
where entry at row $m$ and column $n$ of matrix $\mathbf{K}_{ij}[m, n]$ equals the kernel function evaluated with the row $m$ of $\mathcal{C}^{\mathcal{M}_i}$ and the row $n$ of $\mathcal{C}^{\mathcal{M}_j}$, i.e. $\mathbf{K}_{ij}[m, n] = k(\mathcal{C}^{\mathcal{M}_i}[m], \mathcal{C}^{\mathcal{M}_j}[n])$. Similarly, we define the empirical signed-measure Cosine Mean Similarity ($\mathrm{sCMS}$) between $\mathcal{C}^{\mathcal{M}_1}$ and $\mathcal{C}^{\mathcal{M}_2}$ under kernel function $k(\cdot,\cdot)$ and signed weighting function $w(\cdot)$ as
\begin{align}
    \mathrm{sCMS}_{k}^w\left(\mathcal{C}^{\mathcal{M}_1}, \mathcal{C}^{\mathcal{M}_2}\right) = \frac{w\left(\mathcal{C}^{\mathcal{M}_1}\right)^{\text{T}}\mathbf{K}_{12}w\left(\mathcal{C}^{\mathcal{M}_2}\right)}{\sqrt{w\left(\mathcal{C}^{\mathcal{M}_1}\right)^{\text{T}}\mathbf{K}_{11}w\left(\mathcal{C}^{\mathcal{M}_1}\right)} \cdot \sqrt{w\left(\mathcal{C}^{\mathcal{M}_2}\right)^{\text{T}}\mathbf{K}_{22}w\left(\mathcal{C}^{\mathcal{M}_2}\right)}}
\end{align}

$\mathrm{sMMD}$ and $\mathrm{sCMS}$ extend the traditional $\mathrm{MMD}$ \citep{gretton2012kernel} and $\mathrm{CMS}$ \citep{gruber2024disentangling} defined on probability measures to signed measures covered by the general Reproducing Kernel Hilbert Space (RKHS) theory \citep{sriperumbudur2011universality, simon2018kernel} to accommodate the general RL setting where states and rewards can take negatives values and unnormalised.

We claim that there exists kernel functions $k(\cdot,\cdot)$s and signed weighting functions $w(\cdot)$s, such that the following statements hold:

{
\small
\begin{align}
    \labelAndRemember{mrres1}{&\left\Vert{\Mr^1}' - {\Mr^2}'\right\Vert_2^2 = \mathrm{sMMD}_{k_R}^{w_R}\left(\mathcal{C}^{\mathcal{M}_{1}}, \mathcal{C}^{\mathcal{M}_2}\right)} \\
    \labelAndRemember{mtres1}{&\left\Vert{\Mt^1}' - {\Mt^2}'\right\Vert_F^2 = \mathrm{sMMD}_{k_T}^{w_T}\left(\mathcal{C}^{\mathcal{M}_{1}}, \mathcal{C}^{\mathcal{M}_2}\right)} \\
    \labelAndRemember{mtres11}{&\left\Vert\mathrm{tril}\left({\Mt^1}'{{\Mt^1}'}^{\text{T}}\right) - \mathrm{tril}\left({\Mt^2}'{{\Mt^2}'}^{\text{T}}\right)\right\Vert_2^2 = \mathrm{sMMD}_{k_{TT}}^{w_{TT}}\left(\mathcal{C}^{\mathcal{M}_{1}}, \mathcal{C}^{\mathcal{M}_2}\right)} \\
    \labelAndRemember{mrres2}{&\left\Vert \frac{{\Mr^1}'}{\left\Vert{\Mr^1}' \right\Vert_2} - \frac{{\Mr^2}'}{\left\Vert{\Mr^2}'\right\Vert_2}\right\Vert_2^2 = 2\cdot\left(1-\mathrm{sCMS}_{k_R}^{w_R}\left(\mathcal{C}^{\mathcal{M}_{1}}, \mathcal{C}^{\mathcal{M}_2}\right)\right)} \\
    \labelAndRemember{mtres2}{&\left\Vert \frac{\mathrm{tril}\left({\Mt^1}'{{\Mt^1}'}^{\text{T}}\right)}{\left\Vert \mathrm{tril}\left({\Mt^1}'{{\Mt^1}'}^{\text{T}}\right) \right\Vert_2} - \frac{\mathrm{tril}\left({\Mt^2}'{{\Mt^2}'}^{\text{T}}\right)}{\left\Vert \mathrm{tril}\left({\Mt^2}'{{\Mt^2}'}^{\text{T}}\right) \right\Vert_2}\right\Vert_2^2 = 2\cdot \left(1 - \mathrm{sCMS}_{k_{TT}}^{w_{TT}}\left(\mathcal{C}^{\mathcal{M}_{1}}, \mathcal{C}^{\mathcal{M}_2}\right) \right) }\\
    \recallLabel{finalrep}\\
    &\recallLabel{finalrepunnorm}
\end{align}
}
where $f_{T, R}$ and $\widetilde{f_{T, R}}$ are defined in \Secref{plearning}.

\subsection*{Proof of \Eqref{mtres1}:}
From \Eqref{post},
\begin{align}
    {\Mt^1}'  &= \left({\Ct^1}^{\text{T}}\Ct^{1} + \xit\right)^{-1}{\Ct^{1}}^{\text{T}}\mathbf{S}_1' \\
    {\Mt^2}'  &= \left({\Ct^2}^{\text{T}}\Ct^{2} + \xit\right)^{-1}{\Ct^{2}}^{\text{T}}\mathbf{S}_2'
\end{align}
% Hence,
% \begin{align}
%     {\Mt^1}' - {\Mt^2}' &= \xit^{-1}{\Ct^1}^{\text{T}}\left(\mathbf{I} + \Ct^1\xit^{-1}{\Ct^1}^\text{T} \right)^{-1} \mathbf{S}_1'  - \xit^{-1}{\Ct^2}^{\text{T}}\left(\mathbf{I} + \Ct^2\xit^{-1}{\Ct^2}^\text{T} \right)^{-1}\mathbf{S}_2'
% \end{align}
Let 
\begin{align}
    &\widetilde{\mathbf{S}_1} = \mathbf{S}'_1 \qquad \mathbf{L}_1^\text{T} = \left({\Ct^1}^{\text{T}}\Ct^{1} + \xit\right)^{-1}{\Ct^{1}}^{\text{T}}\\
    &\widetilde{\mathbf{S}_2} = \mathbf{S}'_2
     \qquad
    \mathbf{L}_2^\text{T} = \left({\Ct^2}^{\text{T}}\Ct^{2} + \xit\right)^{-1}{\Ct^{2}}^{\text{T}}
\end{align}
Therefore, the squared Frobenius norm of ${\Mt^1}' - {\Mt^2}'$ is 
\begin{align}
\label{mtmmd}
\begin{split}
    \left\Vert{\Mt^1}' - {\Mt^2}'\right\Vert_F^2 &= \Tr{\left[\left({\Mt^1}' - {\Mt^2}'\right)^\text{T}\left({\Mt^1}' - {\Mt^2}'\right)\right]} \\
    &= \Tr{\left[\widetilde{\mathbf{S}_1}^\text{T}\mathbf{L}_1\mathbf{L}_1^\text{T}\widetilde{\mathbf{S}_1}\right]} + \Tr{\left[\widetilde{\mathbf{S}_2}^\text{T}\mathbf{L}_2\mathbf{L}_2^\text{T}\widetilde{\mathbf{S}_2}\right]} - 2\Tr{\left[\widetilde{\mathbf{S}_1}^\text{T}\mathbf{L}_1\mathbf{L}_2^\text{T}\widetilde{\mathbf{S}_2}\right]} \\
    &= \mathrm{vec}\left({\widetilde{\mathbf{S}_1}}\right)^\text{T} \left( \left(\mathbf{I} \otimes \mathbf{L}_{1}\right)\left(\mathbf{I} \otimes \mathbf{L}_{1}\right)^\text{T} \right)~\mathrm{vec}\left({\widetilde{\mathbf{S}_1}}\right) 
    \\& \quad + \mathrm{vec}\left({\widetilde{\mathbf{S}_2}}\right)^\text{T} \left( \left(\mathbf{I} \otimes \mathbf{L}_{2}\right)\left(\mathbf{I} \otimes \mathbf{L}_{2}\right)^\text{T} \right)~\mathrm{vec}\left({\widetilde{\mathbf{S}_2}}\right) 
    \\& \quad - 2\cdot \mathrm{vec}\left({\widetilde{\mathbf{S}_1}}\right)^\text{T}\left( \left(\mathbf{I} \otimes \mathbf{L}_{1}\right)\left(\mathbf{I} \otimes \mathbf{L}_{2}\right)^\text{T} \right)~\mathrm{vec}\left({\widetilde{\mathbf{S}_2}}\right)
\end{split}
\end{align}
Let $\mathbf{B}_1 = \mathbf{I} \otimes \mathbf{L}_{1}$ and $\mathbf{B}_2 = \mathbf{I} \otimes \mathbf{L}_{2}$. \Eqref{mtres1} is equivalent to
\begin{align}
    \begin{split}
            \left\Vert{\Mt^1}' - {\Mt^2}'\right\Vert_F^2  =  \mathrm{vec}\left({\widetilde{\mathbf{S}_1}}\right) ^{\text{T}} \mathbf{B}_1\mathbf{B}_1^\text{T}  \mathrm{vec}\left({\widetilde{\mathbf{S}_1}}\right)  
            &+\mathrm{vec}\left({\widetilde{\mathbf{S}_2}}\right) ^{\text{T}}\mathbf{B}_2\mathbf{B}_2^\text{T} \mathrm{vec}\left({\widetilde{\mathbf{S}_2}}\right) 
    \\&- 2 \cdot \mathrm{vec}\left({\widetilde{\mathbf{S}_1}}\right) ^{\text{T}}\mathbf{B}_1\mathbf{B}_2^\text{T}  \mathrm{vec}\left({\widetilde{\mathbf{S}_2}}\right) 
    \end{split}
\end{align}
Thus, we have shown
\begin{align}
    \recallLabel{mtres1}
\end{align}
where
\begin{align*}
    w_T(\mathcal{C}^{\mathcal{M}_i}) = \mathrm{vec}\left(\widetilde{\mathbf{S}_i}\right) \qquad k_T(\mathcal{C}^{\mathcal{M}_i}[m], \mathcal{C}^{\mathcal{M}_j}[n]) = \mathbf{B}_{i}[m]^\text{T}\mathbf{B}_{j}[n]
\end{align*}

\subsection*{Proof of \Eqref{mtres11}:}
Define a matrix $\mathbf{D}$ whose entries are zeros or ones that only depends on the value of $D_T$, and $\mathbf{D}~\mathrm{vec}\left({\Mt^1}'{{\Mt^1}'}^{\text{T}}\right) = \mathrm{tril}\left({\Mt^1}'{{\Mt^1}'}^{\text{T}}\right)$, $\mathbf{D}~\mathrm{vec}\left({\Mt^2}'{{\Mt^2}'}^{\text{T}}\right) = \mathrm{tril}\left({\Mt^2}'{{\Mt^2}'}^{\text{T}}\right)$. Let
\begin{align}
    &\widetilde{\mathbf{SS}_1} = \mathbf{S}_1'{\mathbf{S}_1'}^{\text{T}} \qquad \mathbf{L}_1^\text{T} = \left({\Ct^1}^{\text{T}}\Ct^{1} + \xit\right)^{-1}{\Ct^{1}}^{\text{T}}\\
    &\widetilde{\mathbf{SS}_2} = \mathbf{S}_2'{\mathbf{S}_2'}^{\text{T}}
    \qquad \mathbf{L}_2^\text{T} = \left({\Ct^2}^{\text{T}}\Ct^{2} + \xit\right)^{-1}{\Ct^{2}}^{\text{T}} 
\end{align}

\Eqref{mtres11} is hence equivalent to 
\begin{multline}
        \left\Vert\mathrm{tril}\left({\Mt^1}'{{\Mt^1}'}^{\text{T}}\right) - \mathrm{tril}\left({\Mt^2}'{{\Mt^2}'}^{\text{T}}\right)\right\Vert_2^2=\mathrm{vec}\left({\mathbf{L}_1^\text{T}{\mathbf{S}'_1}{\mathbf{S}'_1}^{\text{T}}\mathbf{L}_1}\right)^{\text{T}}\mathbf{D}^{\text{T}}\mathbf{D}~\mathrm{vec}\left({\mathbf{L}_1^\text{T}{\mathbf{S}'_1}{\mathbf{S}'_1}^{\text{T}}\mathbf{L}_1}\right)+
    \\\mathrm{vec}\left({\mathbf{L}_2^\text{T}{\mathbf{S}'_2}{\mathbf{S}'_2}^{\text{T}}\mathbf{L}_2}\right)^{\text{T}}\mathbf{D}^{\text{T}}\mathbf{D}~\mathrm{vec}\left({\mathbf{L}_2^\text{T}{\mathbf{S}'_2}{\mathbf{S}'_2}^{\text{T}}\mathbf{L}_2}\right) -2\cdot\mathrm{vec}\left({\mathbf{L}_1^\text{T}{\mathbf{S}'_1}{\mathbf{S}'_1}^{\text{T}}\mathbf{L}_1}\right)^{\text{T}}\mathbf{D}^{\text{T}}\mathbf{D}~\mathrm{vec}\left({\mathbf{L}_2^\text{T}{\mathbf{S}'_2}{\mathbf{S}'_2}^{\text{T}}\mathbf{L}_2}\right)
\end{multline}

Apply $\mathrm{vec}\left(\mathbf{UVW}\right) = \left(\mathbf{W}^\text{T} \otimes \mathbf{U}\right) \mathrm{vec}(\mathbf{V})$, and let
\begin{align}
    \mathbf{B}_1 = \left(\mathbf{L}_1  \otimes \mathbf{L}_1 \right)~\mathbf{D}^{\text{T}} \qquad \mathbf{B}_2 =  \left(\mathbf{L}_2 \otimes \mathbf{L}_2 \right)~\mathbf{D}^{\text{T}}
\end{align}
\Eqref{mtres11} reduces to
\begin{multline}
\left\Vert\mathrm{tril}\left({\Mt^1}'{{\Mt^1}'}^{\text{T}}\right) - \mathrm{tril}\left({\Mt^2}'{{\Mt^2}'}^{\text{T}}\right)\right\Vert_2^2=
\mathrm{vec}\left(\widetilde{\mathbf{SS}_1}\right)^{\text{T}} \mathbf{B}_1 \mathbf{B}_1^{\text{T}} \mathrm{vec}\left(\widetilde{\mathbf{SS}_1}\right) \\+\mathrm{vec}\left(\widetilde{\mathbf{SS}_2}\right)^{\text{T}} \mathbf{B}_2 \mathbf{B}_2^{\text{T}} \mathrm{vec}\left(\widetilde{\mathbf{SS}_2}\right)  -2\cdot \mathrm{vec}\left(\widetilde{\mathbf{SS}_1}\right)^{\text{T}} \mathbf{B}_1 \mathbf{B}_2^{\text{T}} \mathrm{vec}\left(\widetilde{\mathbf{SS}_2}\right)
\end{multline}
Hence, we have proved
\begin{align}
    \recallLabel{mtres11}
\end{align}
where
\begin{align*}
    w_{TT}\left(\mathcal{C}^{\mathcal{M}_i}\right) =  \mathrm{vec}\left({\widetilde{\mathbf{SS}_i}}\right) \qquad k_{TT}(\mathcal{C}^{\mathcal{M}_i}[m], \mathcal{C}^{\mathcal{M}_j}[n]) = \mathbf{B}_{i}[m]^\text{T}\mathbf{B}_{j}[n]
\end{align*}

\subsection*{Proof of \Eqref{mrres1}:}
This is a degenerate case of \Eqref{mtres1} as $\Mr$ are vectors rather than matrices. Following a similar approach, and let
\begin{align}
    &\widetilde{\mathbf{r}_1} = \mathbf{r}_1  \qquad 
    \mathbf{L}_1^\text{T} = \left({\Cr^1}^{\text{T}}\Cr^{1} + \xir\right)^{-1}{\Cr^{1}}^{\text{T}} \\
    &\widetilde{\mathbf{r}_2} = \mathbf{r}_2 \qquad 
    \mathbf{L}_2^\text{T} = \left({\Cr^2}^{\text{T}}\Cr^{2} + \xir\right)^{-1}{\Cr^{2}}^{\text{T}}
\end{align}
The squared $\mathcal{L}_2$ norm of ${\Mr^2}' - {\Mr^1}'$ is
\begin{align}
    \left\Vert {\Mr^2}' - {\Mr^1}' \right\Vert_2^2 &= \left( {\Mr^2}' - {\Mr^1}'\right)^{\text{T}}\left({\Mr^2}' - {\Mr^1}'\right) \\
    &= \widetilde{\mathbf{r}_1}^\text{T}\mathbf{L}_1\mathbf{L}_1^\text{T}\widetilde{\mathbf{r}_1} + \widetilde{\mathbf{r}_2}^\text{T}\mathbf{L}_2\mathbf{L}_2^\text{T}\widetilde{\mathbf{r}_2} - 2\cdot\widetilde{\mathbf{r}_1}^\text{T}\mathbf{L}_1\mathbf{L}_2^\text{T}\widetilde{\mathbf{r}_2}
\end{align}
Thus, we have shown
\begin{align}
    \recallLabel{mrres1}
\end{align}
where 
\begin{align*}
    w_R(\mathcal{C}^{\mathcal{M}_i}) = \widetilde{\mathbf{r}_i} \qquad k_R(\mathcal{C}^{\mathcal{M}_i}[m], \mathcal{C}^{\mathcal{M}_j}[n]) = \mathbf{L}_{i}[m]^\text{T}\mathbf{L}_{j}[n]
\end{align*}
\subsection*{Proof of \Eqref{mtres2}}
Following the proof of \Eqref{mtres11}, \Eqref{mtres2} is equivalent to
{
\small
\begin{align}
    \label{mtres2tmp}
    \left\Vert \frac{\mathrm{tril}\left({\Mt^1}'{{\Mt^1}'}^{\text{T}}\right)}{\left\Vert \mathrm{tril}\left({\Mt^1}'{{\Mt^1}'}^{\text{T}}\right) \right\Vert_2} - \frac{\mathrm{tril}\left({\Mt^2}'{{\Mt^2}'}^{\text{T}}\right)}{\left\Vert \mathrm{tril}\left({\Mt^2}'{{\Mt^2}'}^{\text{T}}\right) \right\Vert_2}\right\Vert_2^2= 2 - 2\cdot \frac{ \mathrm{vec}\left({\Mt^1}'{{\Mt^1}'}^{\text{T}}\right)^{\text{T}}\mathbf{D}^{\text{T}}{\mathbf{D}~\mathrm{vec}\left({\Mt^2}'{{\Mt^2}'}^{\text{T}}\right)}}{\left\Vert \mathrm{tril}\left({\Mt^1}'{{\Mt^1}'}^{\text{T}}\right) \right\Vert_2\left\Vert \mathrm{tril}\left({\Mt^2}'{{\Mt^2}'}^{\text{T}}\right) \right\Vert_2} 
\end{align}
}
\noindent 
Further reducing \Eqref{mtres2} following the definition of $\mathbf{B}$ and $\widetilde{\mathbf{SS}}$ when proving \Eqref{mtres11}
\begin{align}
    &2 - 2 \cdot \frac{ 
    \mathrm{vec}\left(\widetilde{\mathbf{SS}_1}\right)^{\text{T}} \mathbf{B}_1 \mathbf{B}_2^{\text{T}} \mathrm{vec}\left(\widetilde{\mathbf{SS}_2}\right)}{\sqrt{\mathrm{vec}\left(\widetilde{\mathbf{SS}_1}\right)^{\text{T}} \mathbf{B}_1 \mathbf{B}_1^{\text{T}} \mathrm{vec}\left(\widetilde{\mathbf{SS}_1}\right)}\cdot \sqrt{\mathrm{vec}\left(\widetilde{\mathbf{SS}_2}\right)^{\text{T}} \mathbf{B}_2 \mathbf{B}_2^{\text{T}} \mathrm{vec}\left(\widetilde{\mathbf{SS}_2}\right)}}\\
    =& 2\cdot \left(1 - \mathrm{sCMS}_{k_{TT}}^{w_{TT}}\left(\mathcal{C}^{\mathcal{M}_{1}}, \mathcal{C}^{\mathcal{M}_2}\right) \right) 
\end{align}

\subsection*{Proof of \Eqref{mrres2}}
\begin{align}
    \left\Vert \frac{{\Mr^1}'}{\left\Vert{\Mr^1}' \right\Vert_2} - \frac{{\Mr^2}'}{\left\Vert{\Mr^2}'\right\Vert_2}\right\Vert_2^2 = 2 - 2\cdot \frac{{{\Mr^1}'}^{\text{T}}{\Mr^2}'}{\left\Vert{\Mr^1}'\right\Vert_2\left\Vert{\Mr^2}'\right\Vert_2} 
\end{align}
Following the same definition of $\mathbf{L}$ and ${\widetilde{\mathbf{r}}}$ when proving \Eqref{mrres1}. Then,
\begin{align}
    \left\Vert \frac{{\Mr^1}'}{\left\Vert{\Mr^1}' \right\Vert_2} - \frac{{\Mr^2}'}{\left\Vert{\Mr^2}'\right\Vert_2}\right\Vert_2^2 &= 2 - 2\cdot\frac{\widetilde{\mathbf{r}_1}^\text{T}\mathbf{L}_1\mathbf{L}_2^\text{T}\widetilde{\mathbf{r}_2}}{\sqrt{\widetilde{\mathbf{r}_1}^\text{T}\mathbf{L}_1\mathbf{L}_1^\text{T}\widetilde{\mathbf{r}_1}} \cdot \sqrt{\widetilde{\mathbf{r}_2}^\text{T}\mathbf{L}_2\mathbf{L}_2^\text{T}\widetilde{\mathbf{r}_2}}}\\
    &= 2 \cdot\left(1 - \mathrm{sCMS}_{k_R}^{w_R}\left(\mathcal{C}^{\mathcal{M}_{1}}, \mathcal{C}^{\mathcal{M}_2}\right) \right)
\end{align}

\subsection*{Proof of \Eqref{finalrep}}
The proof is straightforward. \Eqref{finalrep} is equivalent to
\begin{align}
    4 - 2 \cdot \left(\frac{\mathrm{tril}\left({\Mt^1}'{{\Mt^1}'}^{\text{T}}\right)^{\text{T}}\mathrm{tril}\left({\Mt^2}'{{\Mt^2}'}^{\text{T}}\right)}{\left\Vert \mathrm{tril}\left({\Mt^1}'{{\Mt^1}'}^{\text{T}}\right) \right\Vert_2\left\Vert \mathrm{tril}\left({\Mt^2}'{{\Mt^2}'}^{\text{T}}\right) \right\Vert_2} + \frac{{{\Mr^1}'}^{\text{T}}{\Mr^2}'}{\left\Vert{\Mr^1}'\right\Vert_2\left\Vert{\Mr^2}'\right\Vert_2}\right)
\end{align}
Using results from \Eqref{mrres2} and \Eqref{mtres2}, we complete the proof immediately.

\subsection*{Proof of \Eqref{finalrepunnorm}}
$\left\Vert \widetilde{f_{T, R}}\left({\Mt^1}', {\Mr^1}'\right) - \widetilde{f_{T, R}}\left({\Mt^2}', {\Mr^2}'\right) \right\Vert_2^2$ is equal to
\begin{align}
    \begin{split}
    &\mathrm{tril}\left({\Mt^1}'{{\Mt^1}'}^{\text{T}}\right)^{\text{T}} \mathrm{tril}\left({\Mt^1}'{{\Mt^1}'}^{\text{T}}\right) + \mathrm{tril}\left({\Mt^2}'{{\Mt^2}'}^{\text{T}}\right)^{\text{T}}\mathrm{tril}\left({\Mt^2}'{{\Mt^2}'}^{\text{T}}\right)\\
    &+ {{\Mr^1}'}^{\text{T}}{\Mr^1}' + {{\Mr^2}'}^{\text{T}}{\Mr^2}'- 2\cdot \mathrm{tril}\left({\Mt^1}'{{\Mt^1}'}^{\text{T}}\right)^{\text{T}} \mathrm{tril}\left({\Mt^2}'{{\Mt^2}'}^{\text{T}}\right)
     - 2 \cdot {{\Mr^1}'}^{\text{T}}{\Mr^2}'
    \end{split}
\end{align}
For clarity, we define the design matrices $\mathbf{B}_1$, $\mathbf{B}_2$ in the proof of \Eqref{mtres11} and \Eqref{mrres1} as $\mathbf{B}_T^1$, $\mathbf{B}_T^2$ and $\mathbf{B}_R^1$, $\mathbf{B}_R^2$, respectively. Therefore, we obtain
\begin{multline}
\mathrm{vec}\left(\widetilde{\mathbf{SS}_1}\right)^{\text{T}} {\mathbf{B}_T^{1}}{\mathbf{B}_T^{1}}^{\text{T}} \mathrm{vec}\left(\widetilde{\mathbf{SS}_1}\right) + \mathrm{vec}\left(\widetilde{\mathbf{SS}_2}\right)^{\text{T}} {\mathbf{B}_T^{2}}{\mathbf{B}_T^{2}}^{\text{T}} \mathrm{vec}\left(\widetilde{\mathbf{SS}_2}\right) +
 \widetilde{\mathbf{r}_1}^\text{T}{\mathbf{B}_R^1}{\mathbf{B}_R^1}^\text{T}\widetilde{\mathbf{r}_1} \\+ \widetilde{\mathbf{r}_2}^\text{T}{\mathbf{B}_R^2}{\mathbf{B}_R^2}^\text{T}\widetilde{\mathbf{r}_2} - 2\cdot \widetilde{\mathbf{r}_1}^\text{T}{\mathbf{B}_R^1}{\mathbf{B}_R^2}^\text{T}\widetilde{\mathbf{r}_2}
-2 \cdot \mathrm{vec}\left(\widetilde{\mathbf{SS}_1}\right)^{\text{T}} {\mathbf{B}_T^{1}}{\mathbf{B}_T^{2}}^{\text{T}} \mathrm{vec}\left(\widetilde{\mathbf{SS}_2}\right) 
\end{multline}
Let 
{\small
\begin{align}
&\mathbf{sr}_1 = \left[\mathrm{vec}\left(\widetilde{\mathbf{SS}_1}\right)^{\text{T}} \quad  \widetilde{\mathbf{r}_1}^\text{T}\right]^{\text{T}} \qquad \mathbf{sr}_2 = \left[\mathrm{vec}\left(\widetilde{\mathbf{SS}_2}\right)^{\text{T}} \quad  \widetilde{\mathbf{r}_2}^\text{T}\right]^{\text{T}} \\
&\mathbf{K}_{11} = \begin{bmatrix}
    {\mathbf{B}_T^1}{\mathbf{B}_T^1}^{\text{T}} & \mathbf{0} \\
    \mathbf{0} & {\mathbf{B}_R^1}{\mathbf{B}_R^1}^{\text{T}}
\end{bmatrix} \quad \mathbf{K}_{22} = \begin{bmatrix}
    {\mathbf{B}_T^2}{\mathbf{B}_T^2}^{\text{T}} & \mathbf{0} \\
    \mathbf{0} & {\mathbf{B}_R^2}{\mathbf{B}_R^2}^{\text{T}}
\end{bmatrix} \quad \mathbf{K}_{12} = \begin{bmatrix}
    {\mathbf{B}_T^1}{\mathbf{B}_T^2}^{\text{T}} & \mathbf{0} \\
    \mathbf{0} & {\mathbf{B}_R^1}{\mathbf{B}_R^2}^{\text{T}}
\end{bmatrix} 
\end{align}
}
\noindent Thus
\begin{align}
    \left\Vert \widetilde{f_{T, R}}\left({\Mt^1}', {\Mr^1}'\right) - \widetilde{f_{T, R}}\left({\Mt^2}', {\Mr^2}'\right) \right\Vert_2^2 &=\mathbf{sr}_1^{\text{T}}\mathbf{K}_{11}\mathbf{sr}_{1} +  \mathbf{sr}_2^{\text{T}}\mathbf{K}_{22}\mathbf{sr}_{2} - 2 \cdot \mathbf{sr}_1^{\text{T}}\mathbf{K}_{12}\mathbf{sr}_{2} \\
    &= \mathrm{sMMD}_{k_{TTR}}^{w_{TTR}}\left(\mathcal{C}^{\mathcal{M}_1}, \mathcal{C}^{\mathcal{M}_2}\right)
\end{align}
where
\begin{align*}
    w_{TTR}\left(\mathcal{C}^{\mathcal{M}_i}\right) = \mathbf{sr}_i \qquad k_{TTR}(\mathcal{C}^{\mathcal{M}_i}[m], \mathcal{C}^{\mathcal{M}_j}[n]) = \mathbf{K}_{ij}[m, n]
\end{align*}

% \Eqref{mtmmd} demonstrates an interesting result: the $\widetilde{\mathbf{S}}$-weighted Maximum-Mean Discrepency (MMD) between $\mathcal{C}^{\mathcal{M}_1}$ and $\mathcal{C}^{\mathcal{M}_2}$ defined under Gram matrix $\mathbf{I} \otimes \mathbf{K}$ is \textit{strictly equal} to the squared Frobenius norm of the difference in the posterior $\Mt'$. This implies, less formally speaking, that task representations are guaranteed to resemble under similar tasks and diverge under different tasks, so long as the 
\subsection{Implementation Details}
\label{impdetails}
We report the details of our implementations of \nom and other methods. The implementation of \nom is simple with only model networks $\phit, \phir$ and policy networks $\pi^+_{\psi}$. The model networks $\phit, \phir$ are Multi-Layer Perceptrons (MLPs) consisting of \textit{feature} and \textit{mixture} networks. Feature networks convert raw states and actions to features and are shared in $\phit$ and $\phir$. Mixture networks mix the state and action features, further improving the representativeness. The policy network is actor-only for PPO with linear baseline as suggested by \cite{mclean2025meta} in MetaWorld ML10/45, and actor-critic for SAC in MuJoCo tasks.

For reproducing all MuJoCo results, we follow the official implementations in TrMRL, \pearl and \vbad. All results are run with \textsc{gymnasium==1.2.3} and \textsc{mujoco==3.6.0}. For MetaWorld results, we rerun \maml and \rltwo using the more performant implementation provided by \cite{beck2023hypernetworks}, while re-implement and rerun \vbad as the official implementation does not contain MetaWorld environments. We use the tuned hyperparameters from official implementations in \maml, \rltwo and \vbad. For remaining baselines, we use the reported results from \cite{shala2025efficient}.

The table of all related hyperparameters of \nom is shown in \Apref{hyperparam}.

\newpage
\subsection{ML10 Success Rate Comparisons Per-task}
\label{ml10pertask}
\begin{figure}[h]
    \centering
    \begin{subfigure}{0.49\textwidth}
        \includesvg[width=\textwidth]{imgs/ml10_door-close.svg}
        \caption{Door Close}
    \end{subfigure}
    ~
    \begin{subfigure}{0.49\textwidth}
        \includesvg[width=\textwidth]{imgs/ml10_drawer-open.svg}
        \caption{Drawer Open}
    \end{subfigure}
    \\
    \begin{subfigure}{0.49\textwidth}
        \includesvg[width=\textwidth]{imgs/ml10_lever-pull.svg}
        \caption{Lever Pull}
    \end{subfigure}
    ~
    \begin{subfigure}{0.49\textwidth}
        \includesvg[width=\textwidth]{imgs/ml10_sweep-into.svg}
        \caption{Sweep Into}
    \end{subfigure} \\
    ~
    \begin{subfigure}{0.49\textwidth}
        \includesvg[width=\textwidth]{imgs/ml10_shelf-place.svg}
        \caption{Shelf Place}
    \end{subfigure}
    \caption{Testing success rate for each scenario in ML10.}
\end{figure}

\newpage
\subsection{ML45 Success Rate Comparisons Per-task}
\label{ml45pertask}
\begin{figure}[h]
    \centering
    \begin{subfigure}{0.49\textwidth}
        \includesvg[width=\textwidth]{imgs/ml45_door-lock.svg}
        \caption{Door Lock}
    \end{subfigure}
    ~
    \begin{subfigure}{0.49\textwidth}
        \includesvg[width=\textwidth]{imgs/ml45_door-unlock.svg}
        \caption{Door Unlock}
    \end{subfigure}
    \\
    \begin{subfigure}{0.49\textwidth}
        \includesvg[width=\textwidth]{imgs/ml45_hand-insert.svg}
        \caption{Hand Insert}
    \end{subfigure}
    ~
    \begin{subfigure}{0.49\textwidth}
        \includesvg[width=\textwidth]{imgs/ml45_bin-picking.svg}
        \caption{Bin Picking}
    \end{subfigure} \\
    ~
    \begin{subfigure}{0.49\textwidth}
        \includesvg[width=\textwidth]{imgs/ml45_box-close.svg}
        \caption{Box Close}
    \end{subfigure}
    \caption{Testing success rate for each scenario in ML45. \nom achieves nearly $100\%$ testing success rates in both Door Lock and Door Unlock scenarios.}
\end{figure}

\newpage
\subsection{Qualitative Results on Task Identifiability}
\label{taskid}
\begin{figure}[h]
    \centering
    % The vertical line is created by the '|' between the 3rd and 4th columns.
    % The 'm' column type centers the contents vertically.
    \begin{tabular}{ m{0.07\linewidth} m{0.21\linewidth} m{0.21\linewidth} | m{0.21\linewidth} m{0.21\linewidth} }
        \hline \\
        % --- HEADERS ---
        % The \multicolumn{2}{c|}{...} ensures the vertical line continues through the top header
        & \multicolumn{2}{c|}{\textbf{\nom}} & \multicolumn{2}{c}{\textbf{TrMRL}} \\
        & \centering $\text{step} = 0$ & \centering $\text{step} = 5e5$ & \centering $\text{step} = 0$ & \centering\arraybackslash $\text{step} = 5e6$ \\[2mm]
        
        % --- ROW 1 ---
        \textbf{Run 1} & 
        \includesvg[width=\linewidth]{imgs/glibrl_1_0.svg} & 
        \includesvg[width=\linewidth]{imgs/glibrl_2_0.svg} & 
        \includesvg[width=\linewidth]{imgs/trmrl_1_0.svg} & 
        \includesvg[width=\linewidth]{imgs/trmrl_2_0.svg} \\[1mm]
        
        % --- ROW 2 ---
        \textbf{Run 2} & 
        \includesvg[width=\linewidth]{imgs/glibrl_1_1.svg} & 
        \includesvg[width=\linewidth]{imgs/glibrl_2_1.svg} & 
        \includesvg[width=\linewidth]{imgs/trmrl_1_1.svg} & 
        \includesvg[width=\linewidth]{imgs/trmrl_2_1.svg} \\[1mm]

        % --- ROW 3 ---
        \textbf{Run 3} & 
        \includesvg[width=\linewidth]{imgs/glibrl_1_2.svg} & 
        \includesvg[width=\linewidth]{imgs/glibrl_2_2.svg} & 
        \includesvg[width=\linewidth]{imgs/trmrl_1_2.svg} & 
        \includesvg[width=\linewidth]{imgs/trmrl_2_2.svg} \\[1mm]

        % --- ROW 4 ---
        \textbf{Run 4} & 
        \includesvg[width=\linewidth]{imgs/glibrl_1_3.svg} & 
        \includesvg[width=\linewidth]{imgs/glibrl_2_3.svg} & 
        \includesvg[width=\linewidth]{imgs/trmrl_1_3.svg} & 
        \includesvg[width=\linewidth]{imgs/trmrl_2_3.svg} \\[1mm]

        % --- ROW 5 ---
        \textbf{Run 5} & 
        \includesvg[width=\linewidth]{imgs/glibrl_1_4.svg} & 
        \includesvg[width=\linewidth]{imgs/glibrl_2_4.svg} & 
        \includesvg[width=\linewidth]{imgs/trmrl_1_4.svg} & 
        \includesvg[width=\linewidth]{imgs/trmrl_2_4.svg} \\[1mm]
        \\ \hline 
    \end{tabular}

    % \caption{Visual comparison of rollout states across 5 independent runs. A vertical line separates Method 1 and Method 2 for clarity.}
    \caption{PCA projected task representations of \nom and TrMRL for five independent runs. \nom demonstrates its efficiency and accuracy in distinguishing tasks.}
    \label{fig:method_step_comparison_5rows_vline}
\end{figure}
We visualise the task representations of \nom and TrMRL on the \texttt{HalfCheetahVel} benchmark, projected via 2D PCA across five independent runs. To ensure a rigorous baseline, TrMRL is allocated a $10\times$ larger training step budget. Notably, even prior to any training ($\text{step} = 0$), \nom exhibits better task identifiability than fully trained TrMRL at $5e6$ steps due to its exact Bayesian inference. After merely $5e5$ training steps, \nom perfectly disentangles the task representations, accurately mapping the continuous target velocities into a distinct and highly structured latent space. The spherical pattern matches exactly the normalised representation function $f_{T, R}$.  Under \nom, tasks with similar target velocities are similar in the latent space, while tasks with dissimilar target velocities are dissimilar in the latent space. 

\newpage
\subsection{Posterior Collapse in \vbad}
\label{kl}
\begin{figure}[h]
    \centering
    \includesvg[width=\textwidth]{imgs/ml10_kl.svg}
    \caption{Posterior update KL-divergence for \nom and \vbad. \nom demonstrates meaningful posterior updates.}
\end{figure}
To verify if \vbad can learn meaningful task representations, we check the expected KL-divergence between task posteriors and task priors $\mathbb{E}\left[D_{KL}\left(q(\thetat, \thetar|\mathcal{C}_{t+1})~||~q(\thetat, \thetar|\mathcal{C}_t)\right)\right]$, out of 10 runs in the MetaWorld ML10 benchmark \citep{yu2020meta, mclean2025meta}, where $\mathcal{C}_{t+1} = \mathcal{C}_t \cup c_{t+1}$ updates the set of samples $\mathcal{C}_t$ with the sample $c_{t+1}$ at time step $t+1$. \vbad uses a single latent variable to model both transitions and rewards, hence contributing to only one line in the above figure.

Intuitively, if the expected divergence is close to 0, the majority of posterior updates have collapsed to priors, meaning barely any meaningful task representation has been learnt. Clearly from the above figure, \vbad shows lower posterior update magnitude and fails to learn meaningful representations, while \nom demonstrates obvious divergence between posteriors and priors.

\newpage
\subsection{Sensitivity of Latent Task Dimensions}
\label{sensitivity}
{\color{black}
To demonstrate the sensitivity of \nom with respect to latent task dimensions $D_T$ and $D_R$, we perform hyperparameter search in ML10 on (1) $D_T = \left\{ 4, 8, 16, 32 \right\}$ while fixing $D_R = 256$ and (2) $D_R = \left\{32, 64, 128, 256, 512\right\}$ while fixing $D_T = 16$. We compare on (1) the success rate, (2) the predictive error in transitions, and (3) the predictive error in rewards.

\begin{figure}[h]
    \centering
    \begin{subfigure}{0.49\textwidth}
        \includesvg[width=\textwidth]{imgs/T_success_rate.svg}
        \caption{Success Rate (Fixed $D_R$)}
    \end{subfigure}
    ~
    \begin{subfigure}{0.49\textwidth}
        \includesvg[width=\textwidth]{imgs/T_t_loss.svg}
        \caption{Pred. Error in Transitions (Fixed $D_R$)}
    \end{subfigure}
    \\
    \begin{subfigure}{0.49\textwidth}
        \includesvg[width=\textwidth]{imgs/T_r_loss.svg}
        \caption{Pred. Error in Rewards (Fixed $D_R$)}
    \end{subfigure}
    ~
    \begin{subfigure}{0.49\textwidth}
        \includesvg[width=\textwidth]{imgs/R_success_rate.svg}
        \caption{Success Rate (Fixed $D_T$)}
    \end{subfigure}
    \\
    \begin{subfigure}{0.49\textwidth}
        \includesvg[width=\textwidth]{imgs/R_t_loss.svg}
        \caption{Pred. Error in Transitions (Fixed $D_T$)}
    \end{subfigure}
    ~
    \begin{subfigure}{0.49\textwidth}
        \includesvg[width=\textwidth]{imgs/R_r_loss.svg}
        \caption{Pred. Error in Rewards (Fixed $D_T$)}
    \end{subfigure}
    \caption{Sensitivity analysis of latent task dimensions in \nom. }
\end{figure}
In general, \nom shows robust success rates with respect to latent task dimensions $D_T, D_R$, which can be inferred from Figure (a) and (d). We have observed that \nom achieves state-of-the-art performance on ML10 ($\mathbf{29}\%$ success rate) with $D_T = 8$, with the cost of predictive errors. Figure (b) and (f) indicate that as $D_T, D_R$ grows, the corresponding error reduces, offering an efficiency-accuracy trade-off. Figure (c) and (e) are sanity checks that have confirmed transitions do not affect rewards, and vice versa. Overall, $D_R$ are set to be much larger than $D_T$, as reward functions are generally much harder to learn, compared to transition function. 
}

\newpage
\subsection{Ablation Studies}
\label{ablation}

\label{cnorm}
\begin{figure}[h]
    \centering
    \begin{subfigure}{0.49\textwidth}
        \includesvg[width=\textwidth]{imgs/ml10_reg_sr.svg}
        \caption{Success Rate}
    \end{subfigure}
    ~
    \begin{subfigure}{0.49\textwidth}
        \includesvg[width=\textwidth]{imgs/ml10_reg_ml.svg}
        \caption{Predictive Error}
    \end{subfigure}
    \caption{Success rates and predictive errors of \nom with and without regularisation in ML10. }
\end{figure}
Running \nom and its variant without regularisation in the ML10 benchmark, we can tell the regularisations do not change the overall trend in both success rate and prediction error. However, as the number of training step increases, \nom begins to show in (a): higher success rates with narrower CI; in (b): lower prediction error in both transitions and rewards.

\begin{figure}[h]
    \centering
    \begin{subfigure}{0.49\textwidth}
        \centering
        \includesvg[width=\textwidth]{imgs/ml10_ml.svg}
    \end{subfigure}%
    ~
    \begin{subfigure}{0.49\textwidth}
        \centering
        \includesvg[width=\textwidth]{imgs/ml45_ml.svg}
    \end{subfigure}
    \caption{Errors in transition and reward predictions, comparing \nom and \text{GLiBRL\_wo\_NI}. Up: Transitions; Bottom: Rewards; Left: ML10; Right: ML45. \label{lossfig}}
\end{figure}
\nom can be viewed as a generalised, deep BRL version of \alpaca; whereas \alpaca  assumes the model noises $\sigmat = \SigmaT, \sigmar = \SigmaR$ are fully known a priori, \nom performs full Bayesian inference over them. Under the assumption of \alpaca, \Eqref{llhour} reduces to (see \Apref{alpaca})
\begin{align} 
    \labelAndRemember{tllh_simple}{
    \begin{split}
        \log_{\phit, \phir}(\mathcal{C}) = -\frac{1}{2}\sum_{i=1}^M \biggl( D_S\log |\xit'| &- \Tr \left(\SigmaT^{-1} \Mt'^{\text{T}} \xit' \Mt'\right)  \\
         &+ \log |\xir'| - \Tr \left(\SigmaR^{-1} \Mr'^{\text{T}} \xir' \Mr'\right)\biggr) +  \text{const.}
    \end{split}
    }
\end{align}
We studied whether performing Bayesian inference on model noises is necessary for learning accurate transition and reward models. \nom and its variant without noise inference (\text{GLiBRL\_wo\_NI}) are tested with identical hyperparameters on both ML10 and ML45 benchmarks \footnote{They also have the same initial noises. $(\nut\omegat)^{-1} = \SigmaT = 0.025 \cdot \mathbf{I}$ and $(\nur\omegar)^{-1} = \SigmaR = 0.5$.}. The metrics being evaluated are $\mathcal{L}_1$ norms of prediction errors in both transitions (defined as $|\mathbf{S}' - \Ct\Mt'|_1$) and rewards (defined as $|\mathbf{r} - \Cr\Mr'|_1$). \footnote{Comparisons of success rates are not included, as there is no obvious difference.} 

As demonstrated in \Figref{lossfig}, \nom achieves lower prediction errors across both transitions and rewards compared to the \text{GLiBRL\_wo\_NI} which assumes known noises. Both methods become increasingly erroneous in reward predictions with training steps. This is expected, as more steps result in higher success rates, hence increased magnitude of rewards and errors. 

However, the increasing trend of transition errors of \text{GLiBRL\_wo\_NI} is pathological, as magnitudes of states remain relatively bounded and less relevant with the success rate. The lower prediction error of \nom allows better integrations with model-based methods using imaginary samples, whose quality depends highly on the accuracy of the prediction.

\subsection{Marginal Log-likelihood of Normal-Normal}
\label{alpaca}
We prove \Eqref{tllh_simple} has the following form
\begin{align*}
    \recallLabel{tllh_simple}
\end{align*}
\subsection*{Proof:}
The distributions without inferring on the noise are listed as follows:

\textbf{Likelihood:}
\begin{align}
    p_{\phit}(\mathbf{S}_i'|\mathbf{S}_i, \mathbf{A}_i, \thetat) &= \mathcal{MN}\left(\mathbf{S}_i'|\Ct \mut, \mathbf{I}_N,  \SigmaT \in \mathbb{R}^{D_S \times D_S}\right) \\
    p_{\phir}(\mathbf{r}_i|\mathbf{S}_i, \mathbf{A}_i, \mathbf{S}_i', \thetar) &= \mathcal{MN}\left(\mathbf{r}_i|\Cr \mur, \mathbf{I}_N, \SigmaR \in \mathbb{R}^{1 \times 1} \right)
\end{align}

\textbf{Prior:}
\begin{align}
    \begin{split}
         p(\thetat) = p(\mut) =& \mathcal{MN}(\mut|\Mt \in \mathbb{R}^{D_T \times D_S}, \xit^{-1} \in \mathbb{R}^{D_T \times D_T}, \SigmaT )
    \end{split}\\
   \begin{split}
        p(\thetar) = p(\mur) =& \mathcal{MN}(\mur|\Mr\in \mathbb{R}^{D_R \times 1}, \xir^{-1}\in \mathbb{R}^{D_R \times D_R}, \SigmaR) 
   \end{split}
\end{align}

\textbf{Posterior:}
\begin{align}
    p_{\phit}(\thetat|\mathbf{S}_i, \mathbf{A}_i, \mathbf{S}_i') &= \mathcal{MN}(\mut|\Mt', \xit'^{-1}, \SigmaT)  \\
    p_{\phir}(\thetar|\mathbf{S}_i, \mathbf{A}_i, \mathbf{S}_i', \mathbf{r}) &= \mathcal{MN}(\mur|\Mr', \xir'^{-1}, \SigmaR) 
\end{align}
where
\begin{align}
    \begin{split}
         \Mt' &= {\xit'}^{-1} \left[\Ct^\text{T}\mathbf{S}' + \xit \Mt \right]\\
        {\xit'} &=\Ct^\text{T}\Ct + \xit \\
   \end{split}
    \begin{split}
        \Mr' &= {\xir'}^{-1} \left[\Cr^\text{T}\mathbf{r} +  \xir \Mr \right]\\
        {\xir'} &= \Cr^\text{T}\Cr + \xir\\
    \end{split}
\end{align}

Similar to \Apref{llhproof},
\begin{equation}
    \begin{split}
        p_{\phit} ( \mathbf{S}_i'|\mathbf{S}_i, \mathbf{A}_i) = \frac{p_{\phit}(\thetat,  \mathbf{S}_i'|\mathbf{S}_i, \mathbf{A}_i)}{p_{\phit}(\thetat|\mathbf{S}_i, \mathbf{A}_i, \mathbf{S}_i')}
    \end{split}
\end{equation}
As
\begin{align}
    \begin{split}
        &p_{\phit}(\thetat,  \mathbf{S}_i'|\mathbf{S}_i, \mathbf{A}_i) = \frac{|\xit|^{D_S/2}|\SigmaT|^{-D_T/2}}{\sqrt{(2\pi)^{D_TD_S}}} \cdot \exp{\left[ -\frac{1}{2}\Tr\left( \SigmaT^{-1} (\mut - \Mt)^\text{T} \xit  (\mut - \Mt) \right) \right]}\\
        &\qquad\qquad\qquad\qquad\qquad \cdot \frac{|\SigmaT|^{-N/2}}{\sqrt{(2\pi)^{ND_S}}} \cdot \exp{\left[ -\frac{1}{2} \Tr\left( \SigmaT^{-1} (\mathbf{S}_i' - \Ct\mut)^{\text{T}} (\mathbf{S}_i' - \Ct\mut)\right) \right]}
    \end{split}
\end{align}
And
\begin{align}
   p_{\phit}(\thetat|\mathbf{S}_i, \mathbf{A}_i, \mathbf{S}_i') = \frac{|\xit'|^{D_S/2}|\SigmaT|^{-D_T/2}}{\sqrt{(2\pi)^{D_TD_S}}} \cdot \exp{\left[ -\frac{1}{2}\Tr\left( \SigmaT^{-1} (\mut - \Mt')^\text{T} \xit'  (\mut - \Mt') \right) \right]}
\end{align}
Hence
\begin{align}
\begin{split}
        p_{\phit} ( \mathbf{S}_i'|\mathbf{S}_i, \mathbf{A}_i) &\propto |\xit'|^{-D_S/2} \cdot \exp\left[ -\frac{1}{2} \Tr\left( -\SigmaT^{-1}\Mt'^{\text{T}} \xit' \Mt' \right) \right]
\end{split}\\
\begin{split}
    \log p_{\phit} ( \mathbf{S}_i'|\mathbf{S}_i, \mathbf{A}_i) &= -\frac{D_S}{2}\log |\xit'| + \frac{1}{2}  \Tr\left(\SigmaT^{-1}\Mt'^{\text{T}} \xit' \Mt' \right) + \text{const.}  
\end{split}
\end{align}
Similarly,
\begin{align}
    \begin{split}
    \log p_{\phir} ( \mathbf{r}_i|\mathbf{S}_i, \mathbf{A}_i, \mathbf{S}'_i) &= -\frac{1}{2} \log |\xir'| + \frac{1}{2}  \Tr\left(\SigmaR^{-1}\Mr'^{\text{T}} \xir' \Mr' \right)  + \text{const.}
\end{split}
\end{align}
Following \Apref{llhproof},
\begin{multline*}
    \recallLabel{tllh_simple}
\end{multline*}

\newpage
\subsection{Hyperparameters, Runtime and Memory}
\label{hyperparam}
We list all hyperparameters of \nom in the following tables. 

In \texttt{HalfCheetahDir}:
\begin{table*}[h]
    \centering
    \setstretch{1.4}
    \begin{tabular}{l|l|l|l}
        \toprule
         \multicolumn{1}{l}{\textbf{Name}} &  \multicolumn{1}{l}{\textbf{Value}} &  \multicolumn{1}{l}{\textbf{Name}} &  \multicolumn{1}{l}{\textbf{Value}} \\
         \cmidrule{1-4}
         \textbf{policy\_learner} & SAC & \textbf{feat\_out\_activation} & True\\
         \textbf{critic\_layer} & [256, 256] & \textbf{t\_mix\_layers} & [64, 32] \\ \textbf{actor\_layer} & [256, 256, 256] & \textbf{t\_mix\_layernorm} & True\\
         \textbf{policy\_activation} & Tanh & \textbf{t\_mix\_out\_activation} & False \\
         \textbf{policy\_optimiser} & Adam & \textbf{r\_mix\_layers} & [128, 64]\\
         \textbf{actor\_lr/critic\_lr} & 3e-4/4e-4 & \textbf{r\_mix\_layernorm} & True \\
         \textbf{policy\_max\_norm} & 10 & \textbf{r\_mix\_out\_activation} & False \\
         \textbf{policy\_weight\_init} & Xavier & \textbf{t\_reg\_coef} & 5e-3 \\
         \textbf{policy\_bias\_init} & 0 & \textbf{r\_reg\_coef} & 1e-3\\
         \textbf{actor\_logstd\_range} & $[\ln 10^{-6}, \ln 2]$ & \textbf{model\_activation} & ReLU\\
         \textbf{tau} & 5e-3 & \textbf{model\_optimiser} & Adam \\
         \textbf{actor\_grad\_steps} & 500 & \textbf{model\_lr} & 2e-4\\
         \textbf{critic\_grad\_steps} & 500 & \textbf{model\_opt\_max\_norm} & None   \\
         \textbf{policy\_update\_freq} & 200 &  \textbf{model\_grad\_epochs} & 1 \\
         \textbf{init\_alpha} & 1 &\textbf{model\_grad\_steps} & 1 \\
         \textbf{alpha\_lr} & 3e-4 & \textbf{init\_mt} & zeros \\
         \textbf{policy\_bs\_range}& [1, 200] &  \textbf{init\_mr} & zeros\\
         \textbf{s\_feat\_layers} & [64, 32] &  \textbf{init\_xit} & ones\\
         \textbf{s\_feat\_outdim} & 32 & \textbf{init\_xir} & ones \\
         \textbf{s\_feat\_layernorm} & False & \textbf{init\_omegat} & ones  \\
         \textbf{a\_feat\_layers} & [32, 16] & \textbf{init\_omegar} & ones \\
         \textbf{a\_feat\_outdim} & 16 & \textbf{init\_nut} & 22 \\
         \textbf{a\_feat\_layernorm} & False & \textbf{init\_nur} & 2 \\
         \bottomrule
    \end{tabular}
\end{table*}
\newpage
In \texttt{HalfCheetahVel}:
\begin{table*}[h]
    \centering
    \setstretch{1.4}
    \begin{tabular}{l|l|l|l}
        \toprule
         \multicolumn{1}{l}{\textbf{Name}} &  \multicolumn{1}{l}{\textbf{Value}} &  \multicolumn{1}{l}{\textbf{Name}} &  \multicolumn{1}{l}{\textbf{Value}} \\
         \cmidrule{1-4}
         \textbf{policy\_learner} & SAC & \textbf{feat\_out\_activation} & True\\
         \textbf{policy\_layers} & [256, 256] & \textbf{t\_mix\_layers} & [64, 32] \\ \textbf{a\_feat\_out\_activation} & True & \textbf{t\_mix\_layernorm} & True\\
         \textbf{policy\_activation} & Tanh & \textbf{t\_mix\_out\_activation} & False \\
         \textbf{policy\_optimiser} & Adam & \textbf{r\_mix\_layers} & [128, 64]\\
         \textbf{actor\_lr/critic\_lr} & 3e-4/4e-4 & \textbf{r\_mix\_layernorm} & True \\
         \textbf{policy\_max\_norm} & 10 & \textbf{r\_mix\_out\_activation} & False \\
         \textbf{policy\_weight\_init} & Xavier & \textbf{t\_reg\_coef} & 5e-3 \\
         \textbf{policy\_bias\_init} & 0 & \textbf{r\_reg\_coef} & 1e-3\\
         \textbf{actor\_logstd\_range} & $[\ln 10^{-6}, \ln 2]$ & \textbf{model\_activation} & ReLU\\
         \textbf{tau} & 1e-2 & \textbf{model\_optimiser} & Adam \\
         \textbf{actor\_grad\_steps} & 2000 & \textbf{model\_lr} & 2e-4\\
         \textbf{critic\_grad\_steps} & 2000 & \textbf{model\_opt\_max\_norm} & None   \\
         \textbf{policy\_update\_freq} & 200 &  \textbf{model\_grad\_epochs} & 1 \\
         \textbf{init\_alpha} & 0.2 &\textbf{model\_grad\_steps} & 50 \\
         \textbf{alpha\_lr} & 3e-4 & \textbf{init\_mt} & zeros \\
         \textbf{policy\_bs\_range}& [1, 200] &  \textbf{init\_mr} & zeros\\
         \textbf{s\_feat\_layers} & [64, 32] &  \textbf{init\_xit} & ones\\
         \textbf{s\_feat\_outdim} & 32 & \textbf{init\_xir} & ones \\
         \textbf{s\_feat\_layernorm} & False & \textbf{init\_omegat} & ones  \\
         \textbf{a\_feat\_layers} & [32, 16] & \textbf{init\_omegar} & ones \\
         \textbf{a\_feat\_outdim} & 16 & \textbf{init\_nut} & 22 \\
         \textbf{a\_feat\_layernorm} & False & \textbf{init\_nur} & 2 \\
         \bottomrule
    \end{tabular}
\end{table*}
\newpage
In \texttt{AntDir}:
\begin{table*}[h]
    \centering
    \setstretch{1.4}
    \begin{tabular}{l|l|l|l}
        \toprule
         \multicolumn{1}{l}{\textbf{Name}} &  \multicolumn{1}{l}{\textbf{Value}} &  \multicolumn{1}{l}{\textbf{Name}} &  \multicolumn{1}{l}{\textbf{Value}} \\
         \cmidrule{1-4}
         \textbf{policy\_learner} & SAC & \textbf{feat\_out\_activation} & True\\
         \textbf{policy\_layers} & [256, 256] & \textbf{t\_mix\_layers} & [64, 32] \\ \textbf{a\_feat\_out\_activation} & True & \textbf{t\_mix\_layernorm} & True\\
         \textbf{policy\_activation} & Tanh & \textbf{t\_mix\_out\_activation} & False \\
         \textbf{policy\_optimiser} & Adam & \textbf{r\_mix\_layers} & [128, 64]\\
         \textbf{actor\_lr/critic\_lr} & 3e-4/4e-4 & \textbf{r\_mix\_layernorm} & True \\
         \textbf{policy\_max\_norm} & 1 & \textbf{r\_mix\_out\_activation} & False \\
         \textbf{policy\_weight\_init} & Xavier & \textbf{t\_reg\_coef} & 5e-3 \\
         \textbf{policy\_bias\_init} & 0 & \textbf{r\_reg\_coef} & 1e-3\\
         \textbf{actor\_logstd\_range} & $[\ln 10^{-6}, \ln 2]$ & \textbf{model\_activation} & ReLU\\
         \textbf{tau} & 1e-2 & \textbf{model\_optimiser} & Adam \\
         \textbf{actor\_grad\_steps} & 1000 & \textbf{model\_lr} & 2e-4\\
         \textbf{critic\_grad\_steps} & 2000 & \textbf{model\_opt\_max\_norm} & None   \\
         \textbf{policy\_update\_freq} & 400 &  \textbf{model\_grad\_epochs} & 1 \\
         \textbf{init\_alpha} & 0.1 &\textbf{model\_grad\_steps} & 5 \\
         \textbf{alpha\_lr} & 3e-4 & \textbf{init\_mt} & zeros \\
         \textbf{policy\_bs\_range}& [1, 200] &  \textbf{init\_mr} & zeros\\
         \textbf{s\_feat\_layers} & [64, 32] &  \textbf{init\_xit} & ones\\
         \textbf{s\_feat\_outdim} & 32 & \textbf{init\_xir} & ones \\
         \textbf{s\_feat\_layernorm} & False & \textbf{init\_omegat} & ones  \\
         \textbf{a\_feat\_layers} & [32, 16] & \textbf{init\_omegar} & ones \\
         \textbf{a\_feat\_outdim} & 16 & \textbf{init\_nut} & 28 \\
         \textbf{a\_feat\_layernorm} & False & \textbf{init\_nur} & 2 \\
         \bottomrule
    \end{tabular}
\end{table*}

\newpage

We use the same hyperparameters for both ML10 and ML45.

\begin{table*}[h]
    \centering
    \setstretch{1.4}
    \begin{tabular}{l|l|l|l}
        \toprule
         \multicolumn{1}{l}{\textbf{Name}} &  \multicolumn{1}{l}{\textbf{Value}} &  \multicolumn{1}{l}{\textbf{Name}} &  \multicolumn{1}{l}{\textbf{Value}} \\
         \cmidrule{1-4}
         \textbf{policy\_learner} & PPO & \textbf{feat\_out\_activation} & True\\
         \textbf{policy\_layers} & [256, 256] & \textbf{t\_mix\_layers} & [64, 32] \\ \textbf{a\_feat\_out\_activation} & True & \textbf{t\_mix\_layernorm} & True\\
         \textbf{policy\_activation} & Tanh & \textbf{t\_mix\_out\_activation} & False \\
         \textbf{policy\_optimiser} & Adam & \textbf{r\_mix\_layers} & [128, 64]\\
         \textbf{policy\_lr} & 5e-4 & \textbf{r\_mix\_layernorm} & True \\
         \textbf{policy\_opt\_max\_norm} & N/A & \textbf{r\_mix\_out\_activation} & False \\
         \textbf{policy\_weight\_init} & Xavier & \textbf{t\_reg\_coef} & 5e-3 \\
         \textbf{policy\_bias\_init} & 0 & \textbf{r\_reg\_coef} & 1e-3\\
         \textbf{policy\_log\_std\_min} & $\ln 10^{-6}$ & \textbf{model\_activation} & ReLU\\
         \textbf{policy\_log\_std\_max} & $\ln 2$ & \textbf{model\_optimiser} & Adam \\
         \textbf{policy\_grad\_epochs} & 10 & \textbf{model\_lr} & 2e-4\\
         \textbf{policy\_grad\_steps} & 20 & \textbf{model\_opt\_max\_norm} & None   \\
         \textbf{ppo\_clip\_eps} & 0.5 &  \textbf{model\_grad\_epochs} & 1 \\
         \textbf{ppo\_gamma} & 0.99 &\textbf{model\_grad\_steps} & 20 \\
         \textbf{ppo\_gae\_lambda} & 0.95 & \textbf{init\_mt} & zeros \\
         \textbf{ppo\_entropy\_coef }& 5e-3 &  \textbf{init\_mr} & zeros\\
         \textbf{s\_feat\_layers} & [64, 32] &  \textbf{init\_xit} & ones\\
         \textbf{s\_feat\_outdim} & 32 & \textbf{init\_xir} & ones \\
         \textbf{s\_feat\_layernorm} & False & \textbf{init\_omegat} & ones  \\
         \textbf{a\_feat\_layers} & [32, 16] & \textbf{init\_omegar} & ones \\
         \textbf{a\_feat\_outdim} & 16 & \textbf{init\_nut} & 40 \\
         \textbf{a\_feat\_layernorm} & False & \textbf{init\_nur} & 2 \\
         \bottomrule
    \end{tabular}
\end{table*}

\vspace{2em}

{\color{black} \nom is rather efficient in both time and memory. Although all of our experiments are run using A100, we have tested that \nom can run fast on much lower-end GPUs with $8\text{GB}$ memory, such as RTX 3070, with each run costing less than $3$ hours. The runtime does not vary much with changes in $D_T$ and $D_R$, despite the quadratic online inference complexity. }

\newpage
